# Supplementary material for: Flow-Assisted Motion Learning Network for Weakly-Supervised Group Activity Recognition
Source: arXiv:2405.18012 source file (2024-05-28)
Supplement: Supplementary file 1 [file 99_supp.tex]

\clearpage
\setcounter{page}{1}
\setcounter{section}{0}
\setcounter{table}{0}

\setcounter{table}{0}
\setcounter{figure}{0}

\setcounter{equation}{0}
\newpage
\appendix

\section{Additional Formula}
\noindent\textbf{Motion-Aware Actor Encoder attention heads.} In the motion-aware actor encoder, the MHSA generates self-attention on actor features with the following calculation:
%~\cite{Vaswani2017-attention} with
\begin{equation}
    \label{eq:attention}
    \begin{aligned}
    \text{Attention}(Q,K,V) = \text{softmax}(\frac{QK^T}{\sqrt{C}})V,
    \end{aligned}
\end{equation}
\begin{equation}
    \label{eq:MHSA_encoder}
    \begin{aligned}
    \text{MHSA}(Z^l) & =\text{Concat}(\text{head}_1,...,\text{head}_h)\omega^O_{\text{s},l}, \\
    \text{where}\, \text{head}_i & = \text{Attention}(Z^l\omega^Q_{\text{s},l},Z^l\omega^K_{\text{s},l},Z^l\omega^V_{\text{s},l}),
    \end{aligned}
\end{equation}
and $\sqrt{C}$ is the channel dimension, $Z^l$ is the actor feature at layer $l$, and the parameter matrices are $\omega^O_{\text{s},l},\omega^Q_{\text{s},l},\omega^K_{\text{s},l},\omega^V_{\text{s},l}$. Meanwhile, MHCA calculates the cross-attention between flattened feature map and actor features.
\begin{equation}
    \label{eq:MHCA encoder}
    \begin{aligned}
    \text{MHCA}(Z^l,F) & =\text{Concat}(\text{head}_1,...,\text{head}_h)\omega^O_{\text{c},l}, \\
    \text{where}\, \text{head}_i & = \text{Attention}(Z^l\omega^Q_{\text{c},l},F\omega^K_{\text{c},l},F\omega^V_{\text{c},l}),
    \end{aligned}
\end{equation}
the parameter matrices for MHCA are $\omega^O_{\text{s},l},\omega^Q_{\text{s},l},\omega^K_{\text{s},l},\omega^V_{\text{s},l}$. We remove the notation $t$, indicating the time index, for simpler writing. To flatten the extracted feature map, we use a $1 \times 1$ convolution kernel, then flatten it along the spatial dimension. 

\section{Data Augmentation}

\begin{figure}[t]
%\vspace{-8mm}
\begin{minipage}{\linewidth}
\begin{minipage}[b]{0.48\linewidth}
\captionof{table}{Ablation on the flow pre-processing method.}
\setlength{\tabcolsep}{4mm}
\begin{tabular}{c|c|c}
    \toprule
    Flow Proc. & MCA & MPCA  \\
    \midrule
    \xmark  & 77.8\%  & 72.3\%  \\
    \cmark  & 79.1\%  & 76.0\%  \\
    \bottomrule
\end{tabular}
\label{tab:ablation_preprocess_flow}
\end{minipage}
\hfill
\begin{minipage}[b]{0.48\linewidth}
\captionof{table}{Ablation on the weight sharing of actor relation MHSA.}
\setlength{\tabcolsep}{3.5mm}
\begin{tabular}{c|c|c}
    \toprule
    Weight share & MCA & MPCA  \\
    \midrule
    \xmark  & 75.8\%  & 70.5\%  \\
    \cmark  & 79.1\% & 76.0\%  \\
    \bottomrule
\end{tabular}
\label{tab:ablation_weight_share}
\end{minipage}
\end{minipage}
%\vspace{-1.5em}
\end{figure}

\begin{figure}[t]
\begin{center}
\includegraphics[width=\columnwidth]{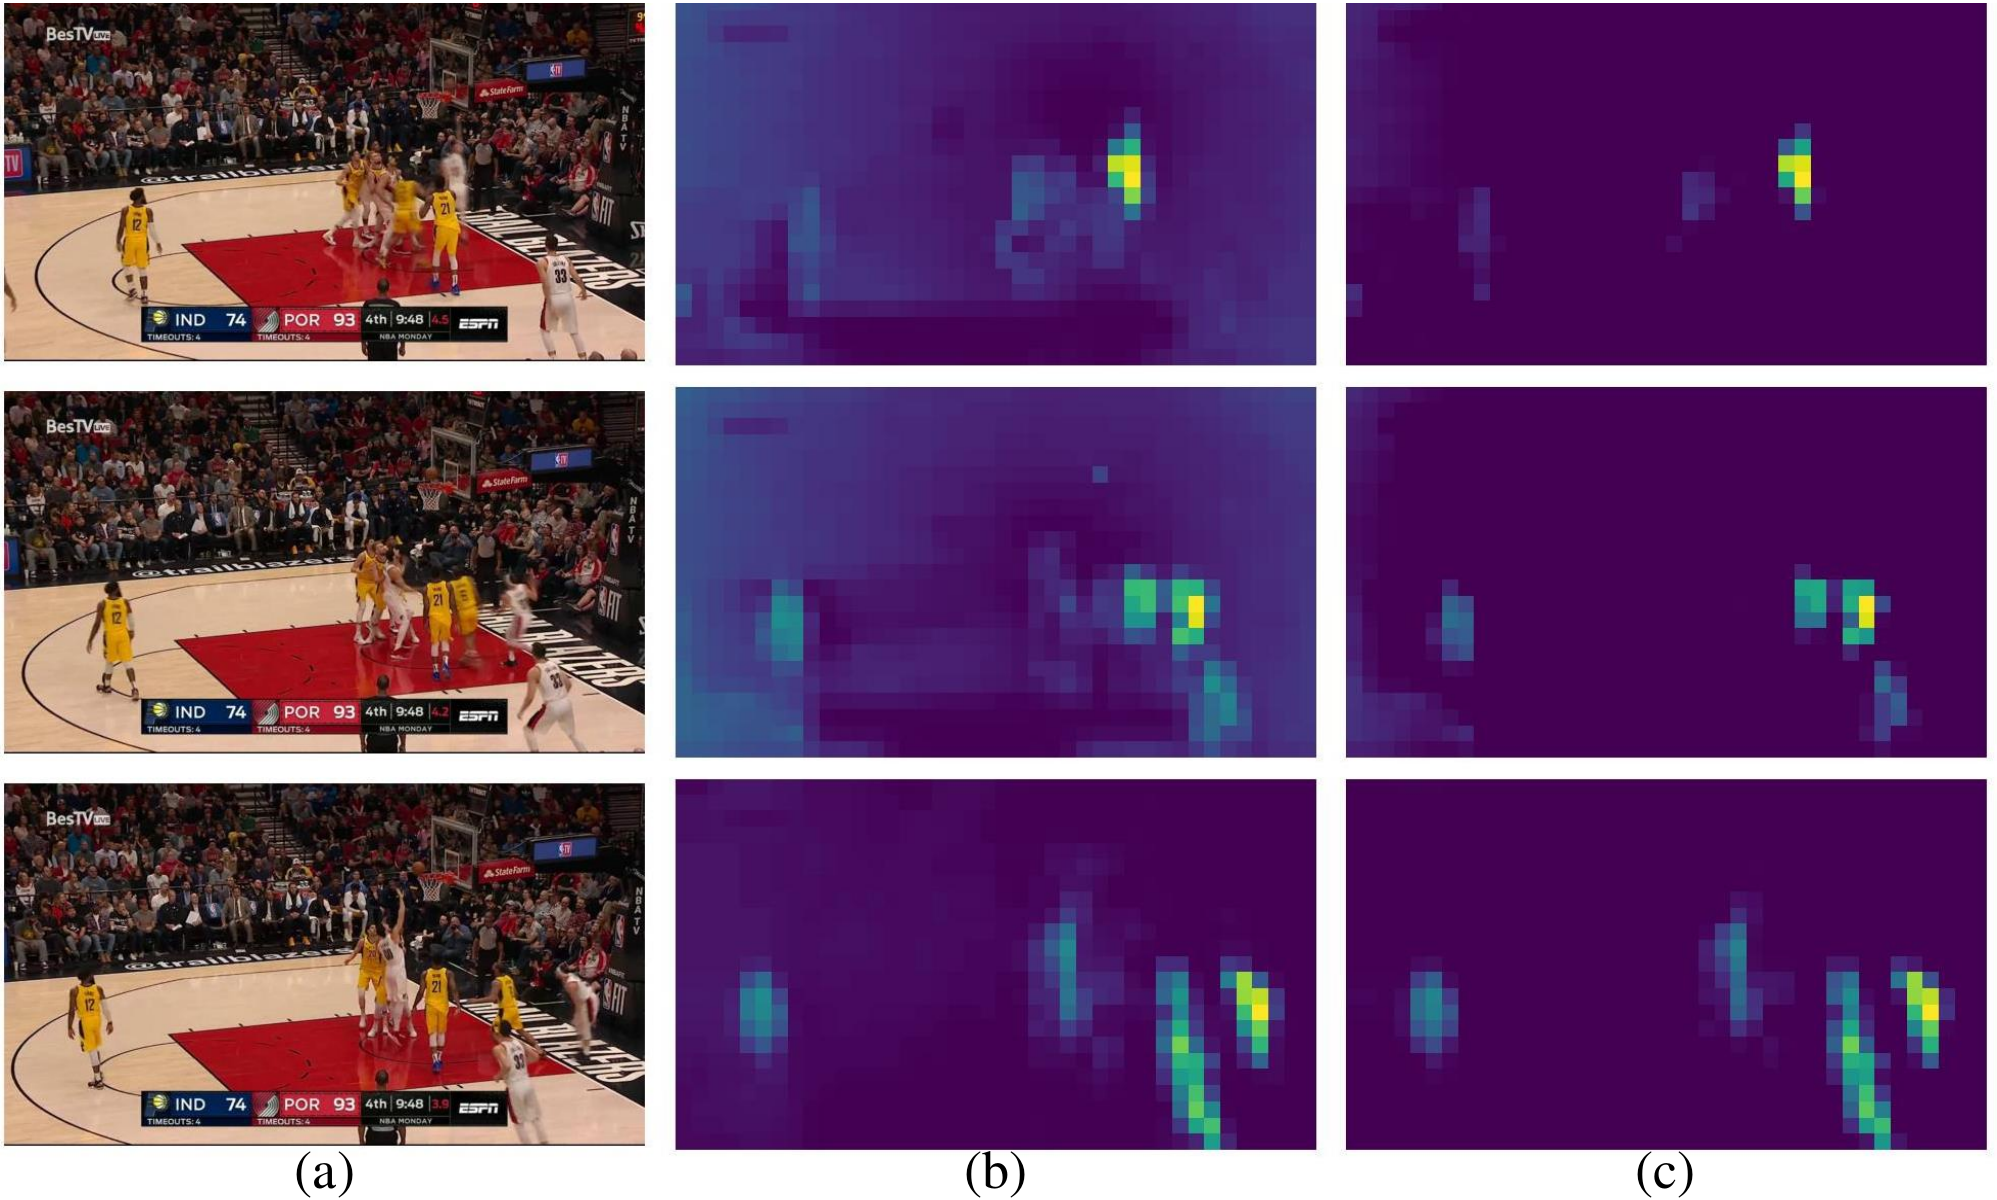}
\end{center}
\vspace{-7mm}
\caption{
From the RGB frames (a), we generate flow map (b) which then we pre-processed into (c) to reduce the effect of camera motion.   
}
\label{fig:supp_fig1}
\vspace{-5mm}
\end{figure}

\noindent\textbf{RGB Frames.}
We perform data augmentation of color jittering and random horizontal flip. For the Volleyball dataset, we also adjust the label when the video frames are flipped horizontally, e.g. \textit{l-pass} to \textit{r-pass}.

\noindent\textbf{Flow maps.}
The optical flow map is extracted frame-per-frame using FlowNet2~\cite{Ilg2017-flownet2} in $1080\times 720$ resolution. Then, we resize it to $W\times H$ matching with the attention map resolution. Additionally, we perform a horizontal flip when the corresponding RGB frames are also flipped. We pre-process the optical flow map to minimize the effect of camera motion in the flow map. Specifically, for each frame, we subtract the value of flow intensity in each pixel with the 85\% quantile value from the whole map. Then, we convert the negative values to zero and normalize the flow map. Figure~\ref{fig:supp_fig1} shows the comparison between the pre-processed flow map and the raw flow map. Table~\ref{tab:ablation_preprocess_flow} shows the performance improvement achieved with this pre-processing.

\section{Additional Ablation Studies}
\noindent\textbf{Actor relation MHSA weight sharing.} In \netnameshort~learning, we share the parameter weight of actor relation MHSA in the actor motion path and group motion path. We performed an ablation study using separate MHSA blocks in the actor and group motion path. In Table~\ref{tab:ablation_weight_share}, the performance of the parameter-sharing model is better than the separate parameter setting.

\noindent\textbf{Configuration of the group motion path.} We perform an ablation study to see the effect of the kernel and stride in the 2D spatio-temporal convolution of the group motion path. From the experiment with results shown in Table~\ref{tab:abl_tempkernel}, we found the optimal configuration of kernel size $5\times3$ and stride $1\times3$ where the first dimension indicates the temporal dimension and the second is the spatial dimension.

\begin{table}[t]
\vspace{2mm}
\caption{Ablation study on spatio-temporal convolution in group motion path.}
\vspace{-4mm}
  \centering
  %\begin{footnotesize}
  \setlength{\tabcolsep}{5mm}{
  
  \resizebox{\columnwidth}{!}{
  \begin{tabular}{l|cc}
  \toprule
  Spatio-temporal Conv. Conf. & MCA & MPCA \\
  \midrule
  Size = $[3 \times 3]$, Stride = $[1 \times 1]$ &\ 78.2\% & 72.7\% \\
  Size = $[3 \times 3]$, Stride = $[1 \times 3]$ &\ 75.7\% & 70.6\% \\
   Size = $[5 \times 3]$, Stride = $[1 \times 1]$ &\ 77.4\% & 72.3\% \\
  \rowcolor{Gray}Size = $[5 \times 3]$, Stride = $[1 \times 3]$ &\ 79.1\% & 76.0\% \\
  Size = $[5 \times 3]$, Stride = $[3 \times 3]$ &\ 74.5\% & 67.9\% \\
  Size = $[5 \times 5]$, Stride = $[1 \times 1]$ &\ 76.5\% & 69.0\% \\
  Size = $[7 \times 3]$, Stride = $[1 \times 3]$ &\ 76.0\% & 72.7\% \\
  %Mirror dual path  &\ \% & \% \\
  %\rowcolor{Gray}\netnameshort &\ \% & \% \\
  \bottomrule
  \end{tabular}}}
   \label{tab:abl_tempkernel}
  %\end{footnotesize}
\vspace{-4mm}
\end{table}

\begin{figure*}[t]
\begin{center}
\includegraphics[width=1.0\textwidth]{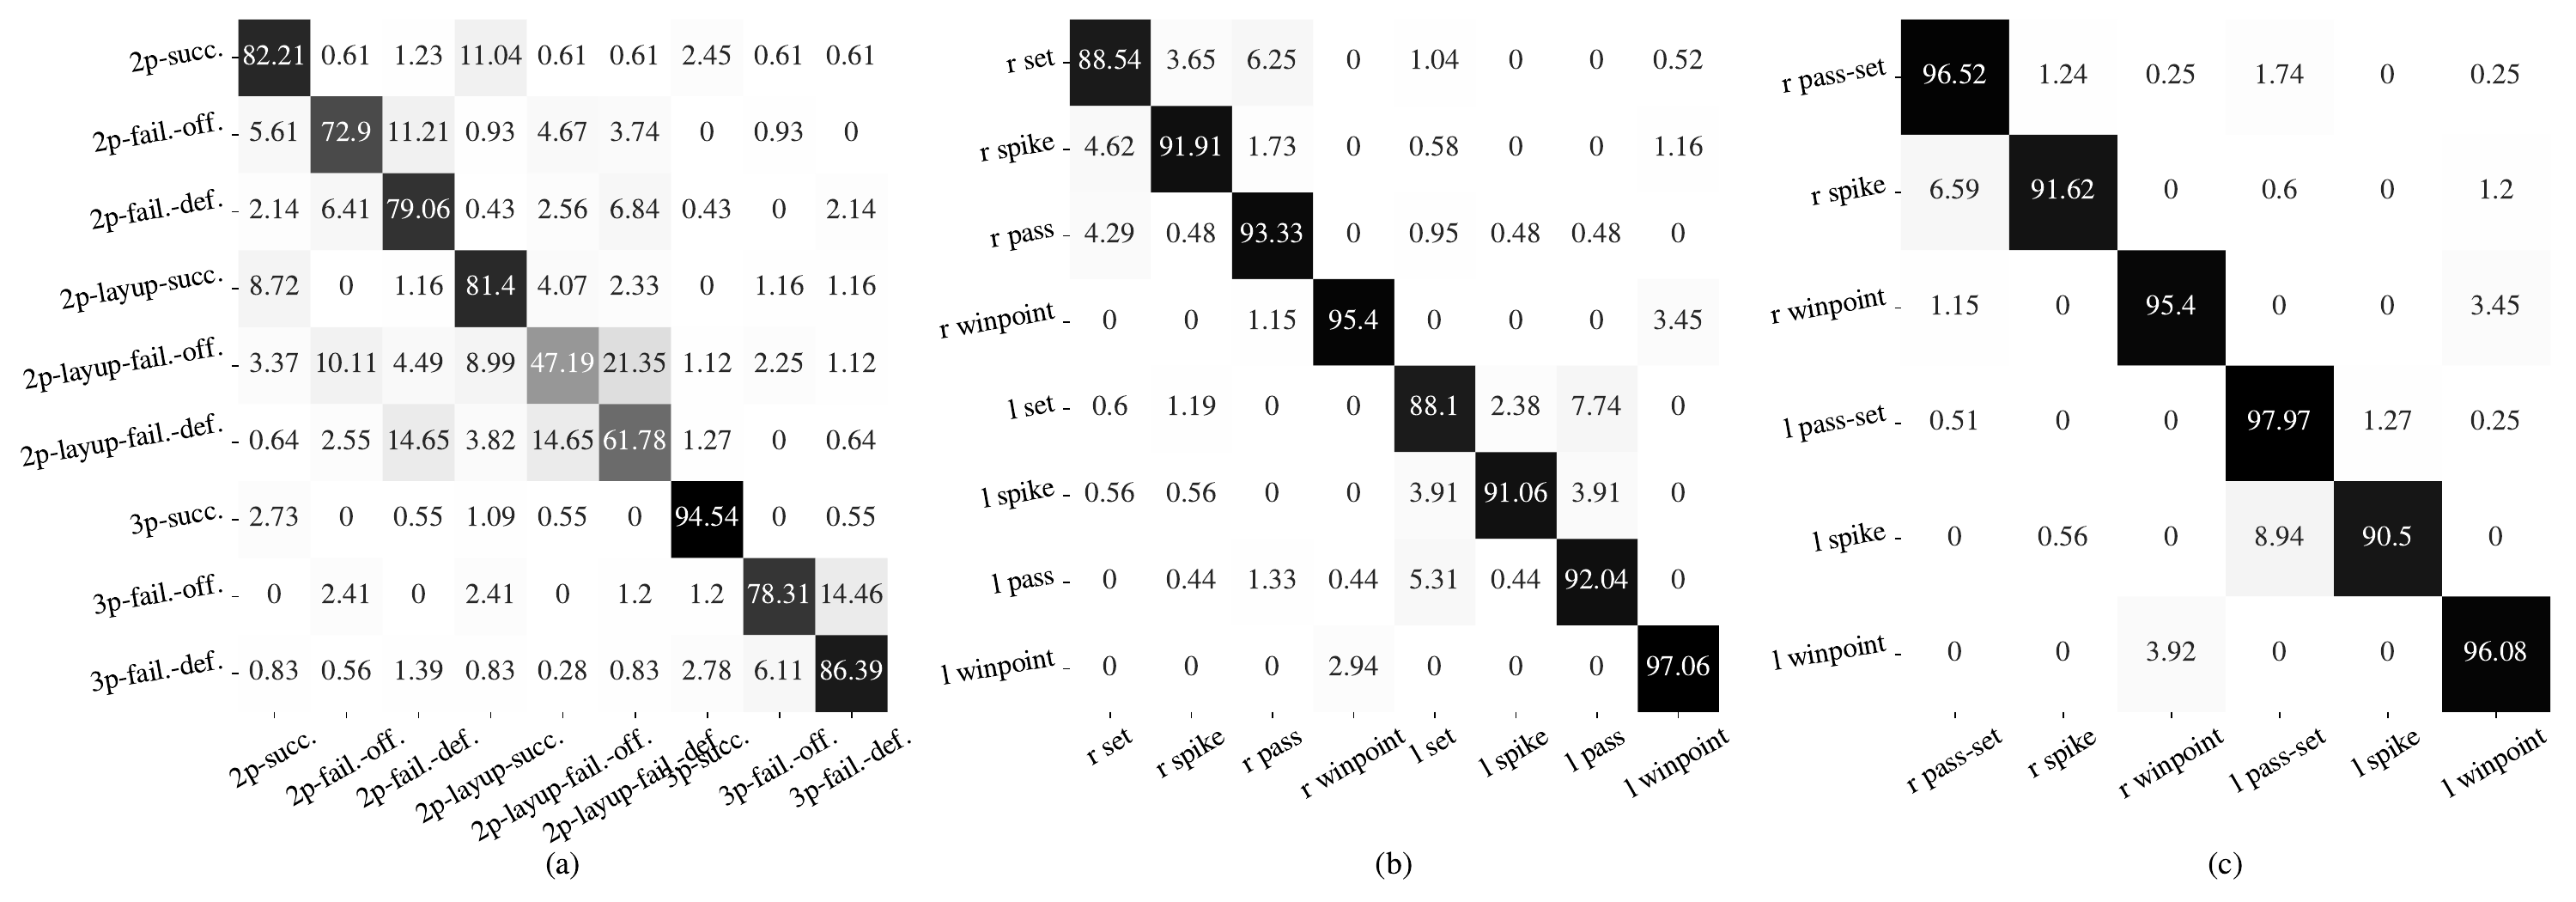}
\end{center}
\vspace{-2em}
\caption{
The confusion matrix (a) on the NBA dataset, (b) of the original 8 class classification on the Volleyball dataset, and (c) of the
merged 6 class classification (merge pass-set class) on the Volleyball dataset.
}
\label{fig:conf_matrix}
%\vspace{-10mm}
\end{figure*}

\section{Additional Experiment Results}
We presented additional qualitative results from the NBA and Volleyball datasets of ResNet-18 variants of Flaming-Net.
Figure~\ref{fig:conf_matrix} shows the confusion matrix on NBA and Volleyball datasets. In (a) \netnameshort~ easily recognizes \textit{2p-succ.} and \textit{3p-succ.} as both classes contain rich visual cues when players react to scored points. Contrastly, \netnameshort~ frequently confuses between \textit{2p-layup-fail-off.} and \textit{2p-layup-fail-def.}. These activities differ in the detail level of which team gets the rebound, which requires the model to understand the context of a team. For the 8 class classification (b), the most confusing cases are \textit{r-set} versus \textit{r-pass} and \textit{l-set} versus \textit{l-pass}. For the merged 6 class classification (c) \netnameshort~ correctly classifies the grouped pass-set class. The confusing cases are then mostly found in differentiating pass-set and spike activity.

Figure~\ref{fig:visualization_nba} and Fig.~\ref{fig:visualization_vb}  show more visualizations of NBA and Volleyball datasets, respectively. For each sample video, we presented three rows where the first row is the RGB frames overlayed with flow maps and the second row is the RGB frames overlayed with motion-aware encoder attention maps. Comparing the attention map with the flow map, we can see that the model only follows the flow guide if the actor is useful to the activity and tends to ignore the influence of irrelevant flow in the background. Lastly, the third row is the visualization of separate token attention maps differentiated by colors. In several frames, we can see that different key actors are highlighted with different tokens. For example, in sample (b) \textit{3p-succ.} of NBA dataset, the token represented by orange color tends to focus on the defending team center, and the shooter is represented with the purple colored token.

\subsection{Experiment Code}
The code to reproduce the experiment is attached with the package file of the supplementary material and will be released to the public after publication.

\subsection{Motion-augmented Backbone}
We use the local motion augmentation in the backbone network adopting from \cite{Kim2022-dfwsgar}. We provide details of the backbone architectures to understand to which place the motion feature modules are inserted. ~\Cref{table:ResNet_detail} and \cref{table:Inception_detail} shows the ResNet-18~\cite{he2016-resnet} and Inception-v3~\cite{szegedy2015-inception} backbone architectures respectively. We insert two motion feature modules after $res_4$ and $res_5$ for the ResNet-18, and after $inc_7$ and $inc_9$ for the Inception-v3.

\begin{figure*}[!t]
\begin{center}
\includegraphics[width=0.91\textwidth]{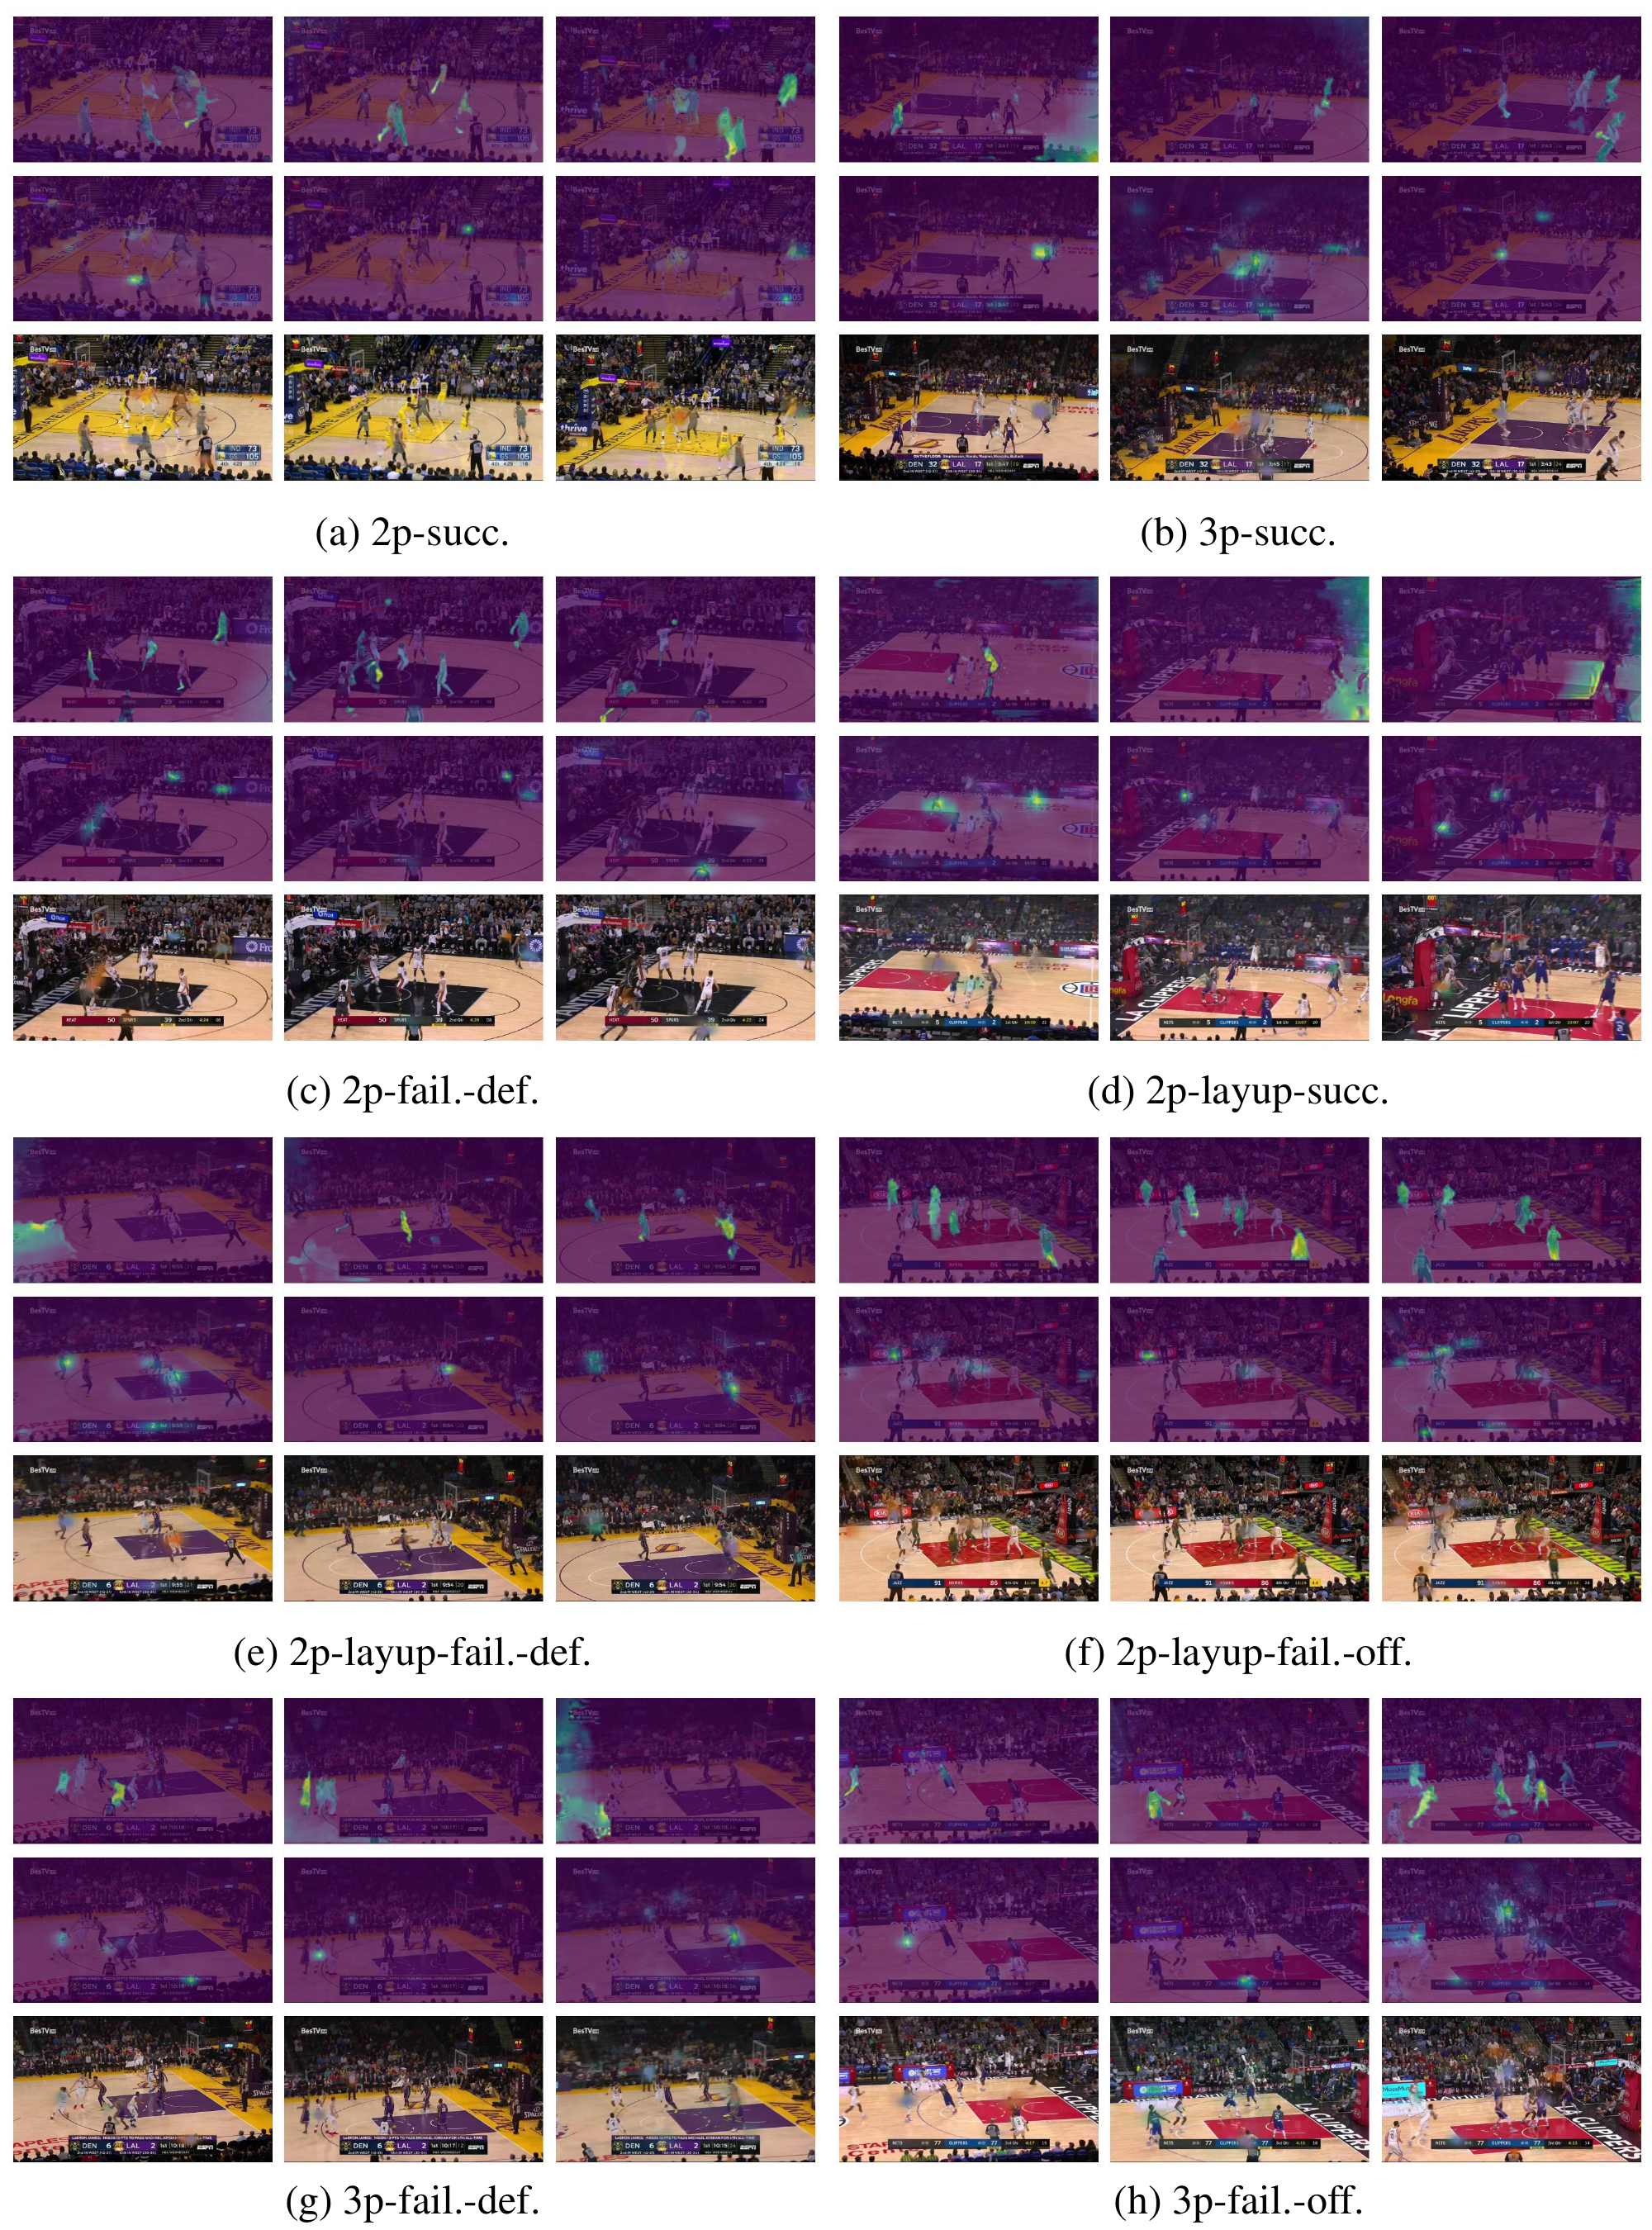}
\end{center}
\vspace{-0.2in}
\caption{Visualizations of the flow-map and cross-attention maps on NBA dataset. For each class, we display in the first row its RGB frames overlayed with the flow map. Then, on the next row, we overlay the RGB frames with the attention map values. Lastly, on the last row, we display separately the attention value of three different tokens to show how our encoder can use different tokens for different actors.}
\label{fig:visualization_nba}
\end{figure*}

\begin{figure*}[!t] \vspace{20pt}
\begin{center}
\includegraphics[width=1.0\linewidth]{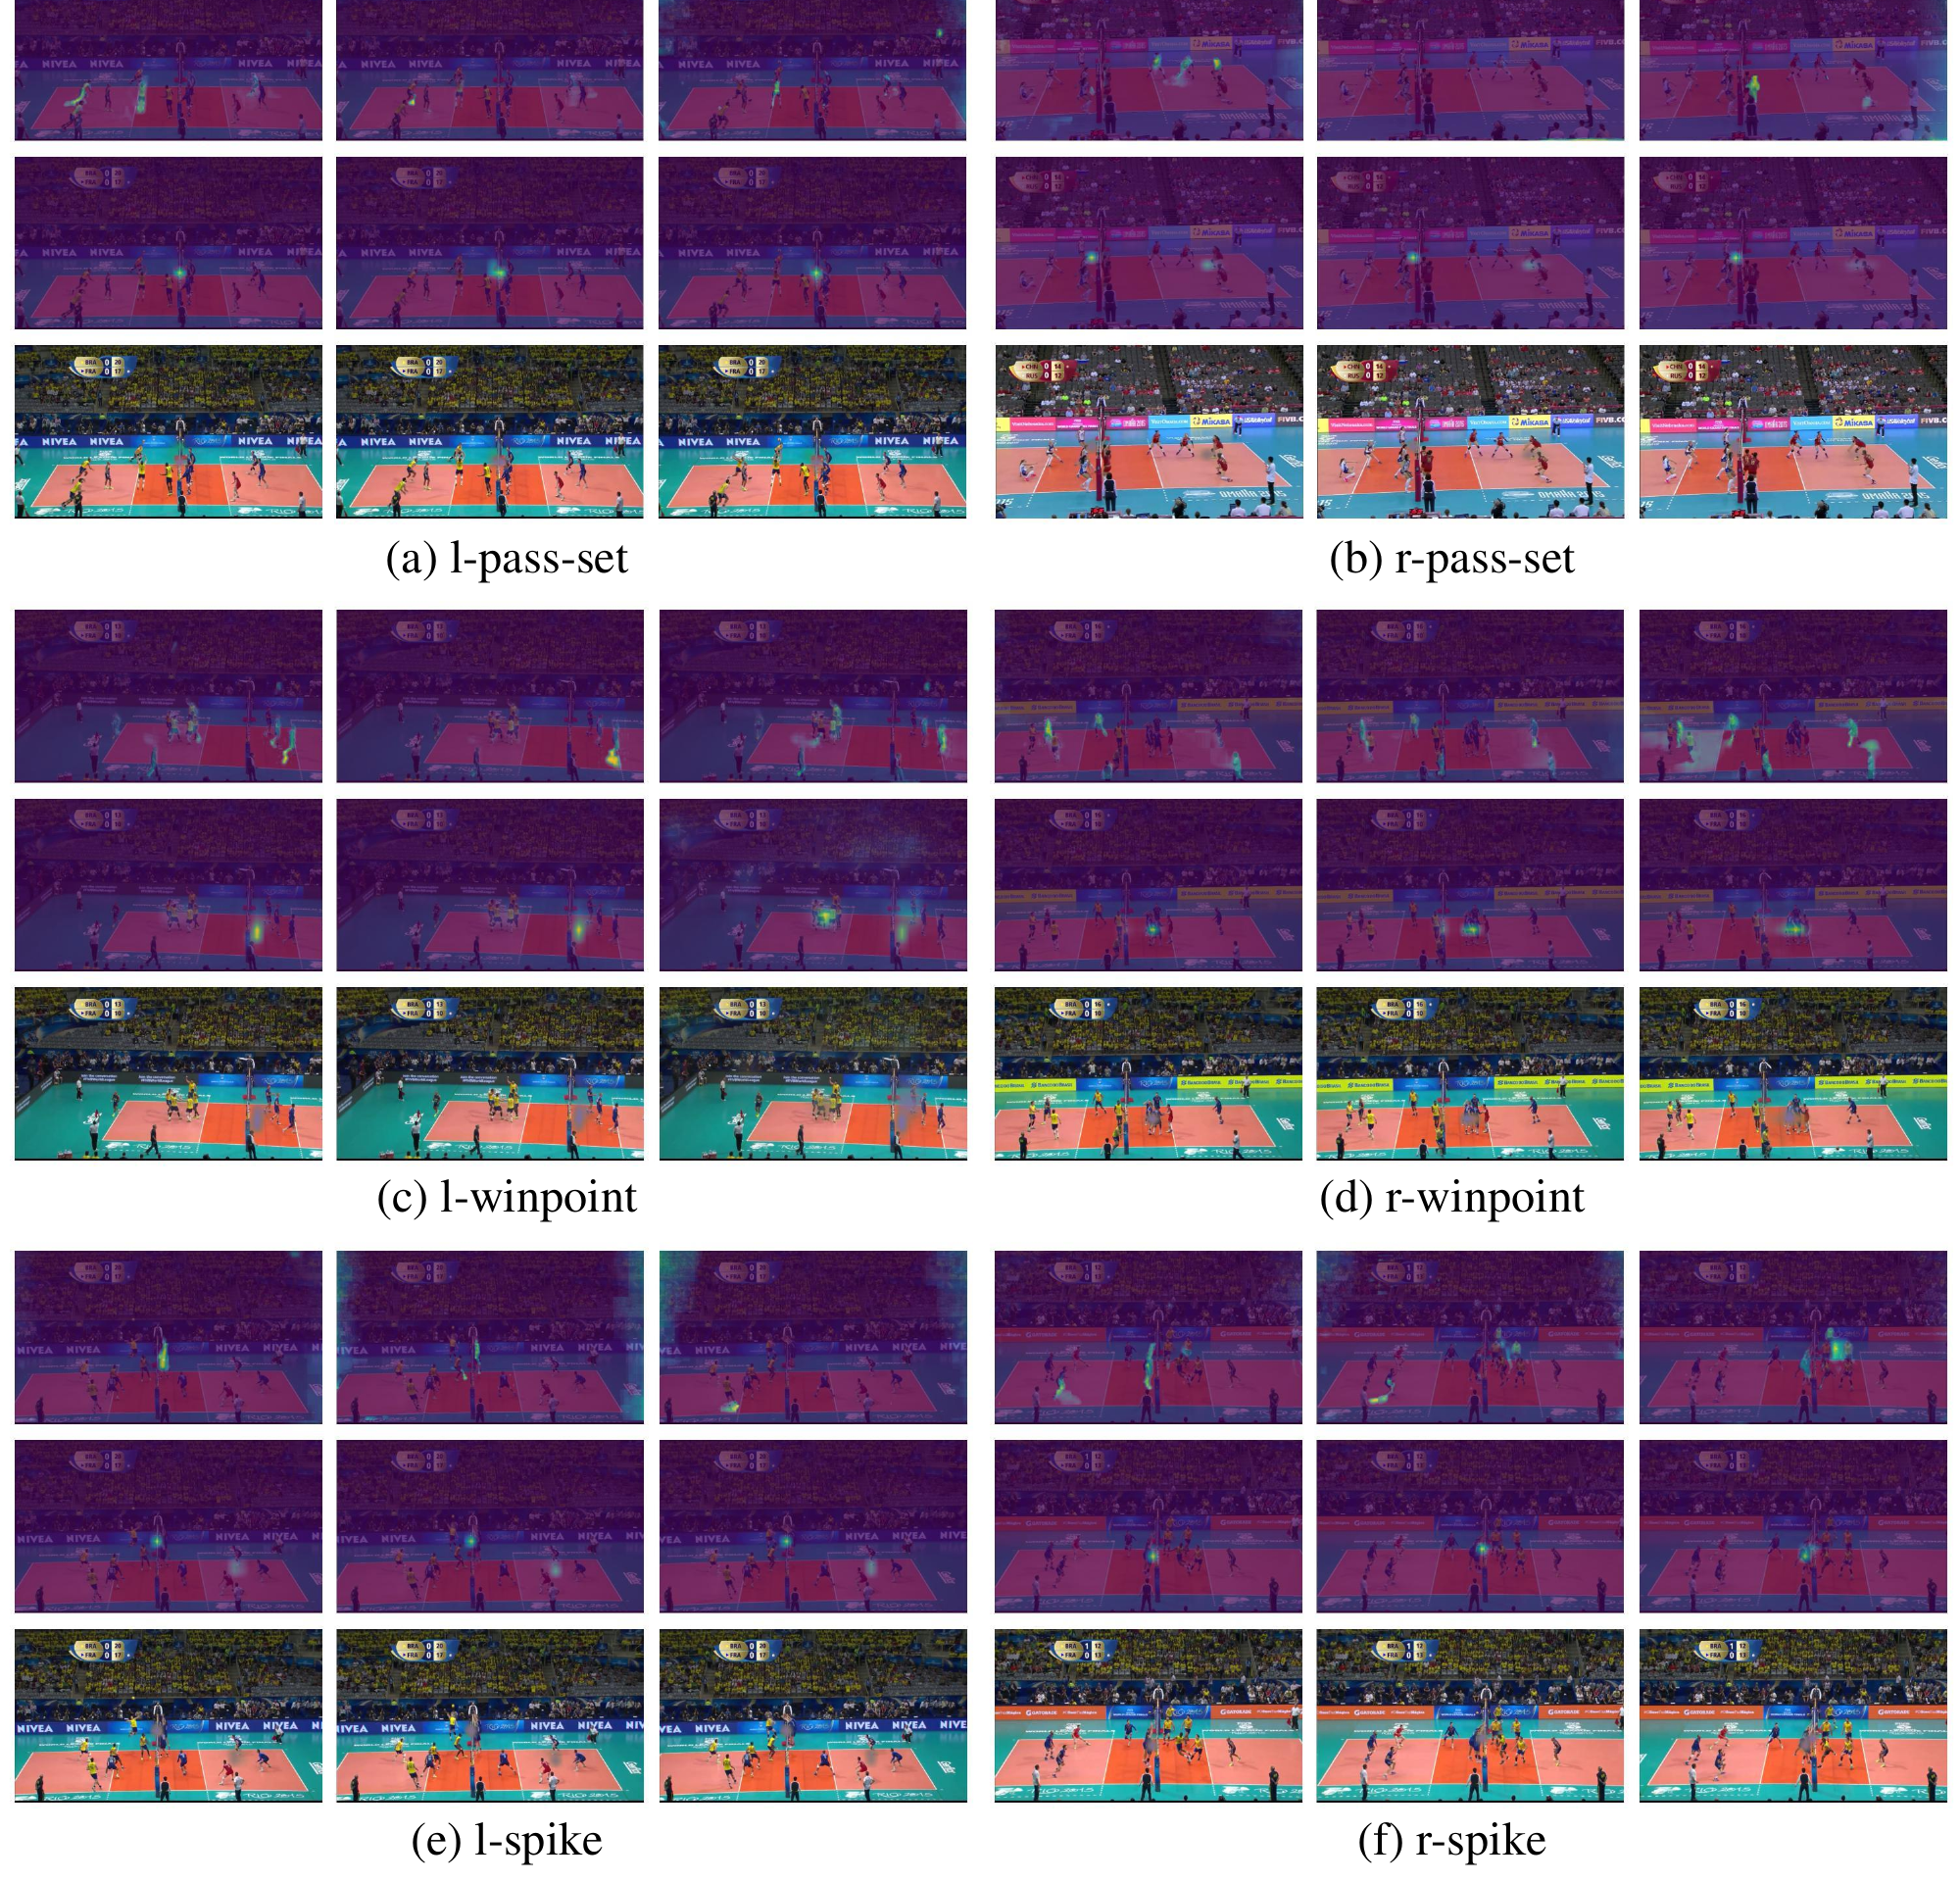}
\end{center}
\caption{Visualizations of the flow-map and cross-attention maps on Volleyball dataset. For each class, we display in the first row its RGB frames overlayed with the flow map. Then, on the next row, we overlay the RGB frames with the attention map values. Lastly, on the last row, we display separately the attention value of three different tokens to show how our encoder can use different tokens for different actors.
\vspace{60pt}}
\label{fig:visualization_vb}
\end{figure*}

\begin{table}[b]
\caption{ResNet-18 backbone details. $[k \times k, c] \times n$ denotes $n$ convolutional layers with kernel size of $k$ and $c$ channels.}
\vspace{-0.2in}
\begin{center}
\setlength{\tabcolsep}{5mm}{

\begin{tabular}{c|c|c}
\hline
Layers & ResNet-18 & Feature map size \\
\hline
\textit{$conv_{1}$}     & $7 \times 7$, 64, stride (2, 2)  & $T \times 360 \times 640$ \\
\hline
\textit{$pool_{1}$}  & $3 \times 3$, stride (2, 2)  & $T \times 180 \times 320$ \\
\hline
\textit{$res_{2}$}  & \bsplitcell{ $3 \times 3$, 64 \\ $3 \times 3$, 64} $\times 2$  & $T \times 180 \times 320$ \\
\hline
\textit{$res_{3}$}  & \bsplitcell{$3 \times 3$, 128 \\ $3 \times 3$, 128} $\times 2$ & $T \times 90 \times 160$ \\
\hline
\textit{$res_{4}$} & \bsplitcell{$3 \times 3$, 256 \\ $3 \times 3$, 256} $\times 2$ & $T \times 45 \times 80$ \\
\hline
\textit{$res_{5}$}  & \bsplitcell{$3 \times 3$, 512 \\ $3 \times 3$, 512} $\times 2$ & $T \times 23 \times 40$ \\
\hline
\end{tabular}
}
\end{center}
\label{table:ResNet_detail}
\vspace{-0.2in}
\end{table}

\begin{table}[t]
%\vspace{-70mm}
\caption{Inception-v3~\cite{szegedy2015-inception} backbone details. $[k \times k, c] \times n$ denotes $n$ convolutional layers with kernel size of $k$ and $c$ channels. We follow the configuration in~\cite{szegedy2015-inception} }
\vspace{-0.2in}
\begin{center}
\setlength{\tabcolsep}{3mm}{

\begin{tabular}{c|c|c}
\hline
Layers & Inception-v3 & Feature map size \\
\hline
\textit{$conv_{1}$}     & $3 \times 3$, 32, stride (2, 2)  & $T \times 32 \times 359 \times 639$ \\
\hline
\textit{$conv_{2}$}     & $3 \times 3$, 32, stride (1, 1)  & $T \times 32 \times 357 \times 637$ \\
\hline
\textit{$conv_{3}$}(padded)     & $3 \times 3$, 64, stride (1, 1)  & $T  \times 64 \times 357 \times 637$ \\
\hline
\textit{$pool_{3}$}  & $3 \times 3$, stride (2, 2)  & $T \times 64 \times 178 \times 318$ \\
\hline
\textit{$conv_{4}$}     & $3 \times 3$, 80, stride (1, 1)  & $T \times 80 \times 176 \times 316$ \\
\hline
\textit{$conv_{5}$}     & $3 \times 3$, 192, stride (2, 2)  & $T \times 192 \times 87 \times 157$ \\
\hline
\textit{$conv_{6}$}     & $3 \times 3$, 288, stride (1, 1)  & $T \times 288 \times 87 \times 157$ \\
\hline
\textit{$inc_{7}$}  & $3 \times$Inception & $T \times 768 \times 43 \times 78$ \\
\hline
\textit{$inc_{8}$}  & $5 \times$Inception & $T \times 1280 \times 21 \times 38$ \\
\hline
\textit{$inc_{9}$} & $2 \times$Inception & $T \times 2048 \times 21 \times 38$ \\
\hline
\end{tabular}
}
\end{center}
\label{table:Inception_detail}
\vspace{-0.2in}
\end{table}
